# Supplementary material for: Harnessing Scale and Physics: A Multi-Graph Neural Operator Framework for PDEs on Arbitrary Geometries
Source: arXiv:2411.15178 source file (2025-02-07)
Supplement: Supplementary file 1 [file 3_implementation_details.tex]

\section{Implementation Details} \label{appendix:config}

\begin{table*}[ht]
\vspace{-10pt}
\centering
\caption{Details of hyperparameters used for benchmarks.}
\label{table:config}

\begin{sc}
    
    \vspace{-5pt}
    \resizebox{0.98\linewidth}{!}{
    \begin{tabular}{c|cccccc}
       \toprule
       Type & NS & Shape-Net Car & Poisson & Cylinder Flow & DP & Airfoil \\
       \midrule
        input\_features  & 1    & 4    & 1    & 3    & 1    & 4    \\
        output\_features & 1    & 4    & 1    & 3    & 1    & 4    \\
        feature\_width   & 128  & 128  & 128  & 128  & 128  & 128  \\
        pos\_dim         & 2    & 3    & 2    & 2    & 3    & 2    \\
        num\_layers      & 3    & 3    & 3    & 3    & 2    & 3    \\
        activation          & 'relu'        & 'relu'        & 'relu'  & 'relu'        & 'relu'          & 'relu'  \\
        batch\_norm      & TRUE & TRUE & TRUE & TRUE & TRUE & TRUE \\
        global\_ratio    & 0.25 & 0.25 & 0.25 & 0.25 & 0.1  & 0.25    \\
        global\_k        & 4    & 4    & 4    & 4    & 3    & 4    \\
        local\_nodes     & 1024 & 512  & 512  & 1024 & 128  & 512  \\
        local\_k         & 6    & 6    & 6    & 6    & 6    & 6    \\
        num\_phys        & 32   & 32   & 32   & 32   & 32   & 32   \\
        num\_heads       & 8    & 8    & 8    & 8    & 8    & 8   \\
       \bottomrule
    \end{tabular}}
\end{sc}
\vspace{-5pt}
\end{table*}

The primary configurations for the AMG, as applied across various benchmarks, are detailed in Table \ref{table:config}.
